# Supplementary material for: Experimental Characterization of the Passive Mechanical Behavior of Rat Pelvic Floor Muscles: Effects of Test Conditions and Pregnancy
Source: arXiv:2609.26871 source file (2026-09-22)
Supplement: Supplementary file 1 [file Abstract_Elsevier.tex]

\textit{Purpose:} Pelvic floor muscles undergo large deformations during vaginal delivery, yet the passive tensile behavior of pregnant and non-pregnant pelvic floor muscle and the influence of testing protocols remain incompletely characterized. This study evaluated how pregnancy, loading rate, preconditioning, and storage affect passive tensile mechanics of rat pelvic floor muscle.

\textit{Methods:} Levator ani samples from pregnant and non-pregnant rats were tested in uniaxial tension to failure across multiple preconditioning amplitudes, two loading rates, and fresh or frozen storage conditions. Peak and transition metrics, strain energy density, toe-region stiffness, and high-strain stiffness were extracted using automated region-detection methods. Rat properties were also compared with digitized human cadaver levator ani data.

\textit{Results:} Pregnant rat samples reached greater peak strains than controls (1.91 $\pm$ 0.60 vs. 1.47 $\pm$ 0.33), although the difference was not significant. Preconditioning affected peak strain in a loading-rate-dependent manner: responses tapered near 2\% preconditioning strain at 0.5\% strain/s, whereas no comparable tapering occurred through 15\% at 1\% strain/s. Compared with human cadaver data, rat samples reached substantially larger peak strains (1.47 $\pm$ 0.33 vs. 0.23 $\pm$ 0.12) and lower high-strain stiffness (90 $\pm$ 66 vs. 105 $\pm$ 48 kPa).

\textit{Conclusion:} This study provides one of the first direct experimental comparisons of passive pelvic floor muscle mechanics between pregnant and non-pregnant tissue, while systematically evaluating how multiple testing-protocol variables influence the measured response. Distinguishing protocol-dependent variability from biological differences provides a more reproducible basis for cross-study comparison and constitutive model calibration. Rat pelvic floor muscle is a useful model for pregnancy-associated adaptation, but absolute mechanical values should be translated to human tissue cautiously.
