# Supplementary material for: Experimental Characterization of the Passive Mechanical Behavior of Rat Pelvic Floor Muscles: Effects of Test Conditions and Pregnancy
Source: arXiv:2609.26871 source file (2026-09-22)
Supplement: Supplementary file 2 [file Graphical_Abstract.tex]

\begin{figure}[htbp!]
    \includegraphics[width=1\textwidth]{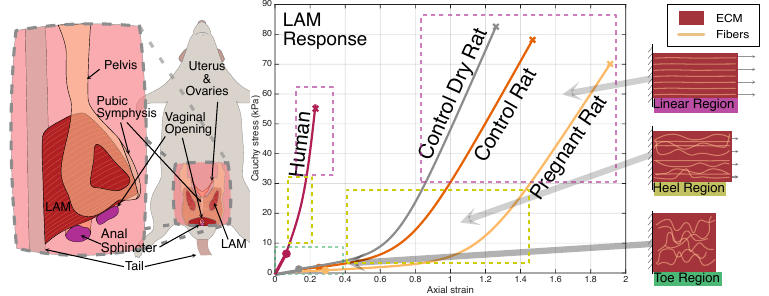}
    \caption*{}
    \label{fig:GraphicalAbstract}
\end{figure}
