# Supplementary material for: Experimental Characterization of the Passive Mechanical Behavior of Rat Pelvic Floor Muscles: Effects of Test Conditions and Pregnancy
Source: arXiv:2609.26871 source file (2026-09-22)
Supplement: Supplementary file 3 [file Highlights.tex]

\section*{Highlights}
\begin{itemize}
    \item Rat pelvic floor mechanics were quantified across controlled testing conditions
    \item Automated detection captured toe stiffness, transition point, and high-strain stiffness 
    \item Mechanical responses varied with preconditioning and loading conditions 
    \item Pregnant rat tissue tended to reach higher strains before failure
    \item Comparing results with published data for human pelvic floor mechanics shows clear species differences
\end{itemize}
